# Supplementary material for: Optimization for Medical Image Segmentation: Theory and Practice when evaluating with Dice Score or Jaccard Index
Source: arXiv:2010.13499 source file (2020-10-26)
Supplement: Supplementary file 3 [file crop_results_stderr.tex]

\begin{tabularx}{\linewidth}{llXYYYYY}
    \toprule
         & Loss & \multicolumn{1}{r}{\lapbox[\width]{1em}{\emph{Dataset} $\rightarrow$}} & 0.1 & 0.2 & 0.3 & 0.4 & 0.5 \\
    \midrule
\parbox[t]{3mm}{\centering\multirow{2}{*}{\rotatebox[origin=c]{90}{Dice}}}
      & CE    & &  0.010 &  0.009 &  0.009 &  0.009 &  0.008 \\
      & sDice & &  0.009 &  0.009 &  0.009 &  0.008 &  0.008 \\
    \midrule
    \parbox[t]{3mm}{\centering\multirow{2}{*}{\rotatebox[origin=c]{90}{Jacc.}}}
      & CE    & &  0.009 &  0.009 &  0.009 &  0.009 &  0.009 \\
      & sDice & &  0.009 &  0.009 &  0.009 &  0.008 &  0.008 \\
         
    \bottomrule
\end{tabularx}
