# Supplementary material for: Optimization for Medical Image Segmentation: Theory and Practice when evaluating with Dice Score or Jaccard Index
Source: arXiv:2010.13499 source file (2020-10-26)
Supplement: Supplementary file 4 [file empirical_results_stderr.tex]

% Std Error
\begin{tabularx}{\linewidth}{lsXYYYYY}
    \toprule
    & & \multicolumn{1}{r}{\lapbox[\width]{1em}{\emph{group} $\rightarrow$}} & \multicolumn{2}{c}{CE-based} & \multicolumn{3}{c}{Metric-sensitive} \\
    \midrule
    & Dataset & \multicolumn{1}{r}{\lapbox[\width]{1em}{\emph{loss} $\rightarrow$}} & CE & wCE & sDice & sJaccard & Lov\'{a}sz \\
    \midrule
    \parbox[t]{7mm}{\centering\multirow{5}{*}{\rotatebox[origin=c]{90}{Dice}}} 
    & BR18 &        & 0.007 & 0.008 & 0.006 & 0.007 & 0.006 \\
    & IS17 &        & 0.039 & 0.039 & 0.034 & 0.035 & 0.038 \\
    & IS18 &        & 0.029 & 0.026 & 0.027 & 0.027 & 0.028 \\
    & MO18 &        & 0.003 & 0.005 & 0.003 & 0.003 & 0.002 \\
    & PO18 &        & 0.010 & 0.009 & 0.009 & 0.010 & 0.010 \\
    & WM17 &        & 0.023 & 0.029 & 0.019 & 0.020 & 0.020 \\
    & WM17\textsuperscript{DM} &        & 0.022 & 0.034 & 0.019 & 0.020 & 0.021 \\
    \midrule
    \parbox[t]{7mm}{\centering\multirow{5}{*}{\rotatebox[origin=c]{90}{Jaccard}}}
    & BR18 &        & 0.009 & 0.009 & 0.008 & 0.008 & 0.008 \\
    & IS17 &        & 0.029 & 0.030 & 0.027 & 0.028 & 0.029 \\
    & IS18 &        & 0.025 & 0.023 & 0.023 & 0.024 & 0.024 \\
    & MO18 &        & 0.004 & 0.006 & 0.004 & 0.004 & 0.004 \\
    & PO18 &        & 0.009 & 0.008 & 0.009 & 0.009 & 0.009 \\
    & WM17 &        & 0.024 & 0.025 & 0.021 & 0.022 & 0.022 \\
    & WM17\textsuperscript{DM} &        & 0.024 & 0.029 & 0.021 & 0.022 & 0.023 \\
    \bottomrule
\end{tabularx}

% IQR
% \begin{tabularx}{\linewidth}{lsXYYYYY}
%     \toprule
%     & & \multicolumn{1}{r}{\lapbox[\width]{1em}{\emph{group} $\rightarrow$}} & \multicolumn{2}{c}{CE-based} & \multicolumn{3}{c}{Metric-sensitive} \\
%     \midrule
%     & Dataset & \multicolumn{1}{r}{\lapbox[\width]{1em}{\emph{loss} $\rightarrow$}} & CE & wCE & sDice & sJaccard & Lov\'{a}sz \\
%     \midrule
%     \parbox[t]{7mm}{\centering\multirow{5}{*}{\rotatebox[origin=c]{90}{Dice}}} 
%     &BR18 &        & 0.097 & 0.134 & 0.081 & 0.083 & 0.084 \\
%     &IS17 &        & 0.466 & 0.473 & 0.335 & 0.357 & 0.421 \\
%     &IS18 &        & 0.479 & 0.322 & 0.324 & 0.318 & 0.379 \\
%     &MO18 &        & 0.029 & 0.054 & 0.031 & 0.031 & 0.029 \\
%     &PO18 &        & 0.462 & 0.385 & 0.389 & 0.395 & 0.417 \\
%     &WM17 &        & 0.228 & 0.291 & 0.186 & 0.186 & 0.176 \\
%     &WM17\textsuperscript{DM} &        & 0.238 & 0.456 & 0.195 & 0.203 & 0.215 \\   
%     \midrule
%     \parbox[t]{7mm}{\centering\multirow{5}{*}{\rotatebox[origin=c]{90}{Jaccard}}}
%     &BR18 &        & 0.152 & 0.197 & 0.130 & 0.135 & 0.137 \\
%     &IS17 &        & 0.304 & 0.344 & 0.251 & 0.270 & 0.309 \\
%     &IS18 &        & 0.422 & 0.295 & 0.317 & 0.310 & 0.356 \\
%     &MO18 &        & 0.053 & 0.093 & 0.056 & 0.057 & 0.053 \\
%     &PO18 &        & 0.537 & 0.426 & 0.472 & 0.477 & 0.500 \\
%     &WM17 &        & 0.269 & 0.259 & 0.229 & 0.231 & 0.215 \\
%     &WM17\textsuperscript{DM} &        & 0.280 & 0.354 & 0.243 & 0.252 & 0.264 \\
%     \bottomrule
% \end{tabularx}
