# Supplementary material for: Optimization for Medical Image Segmentation: Theory and Practice when evaluating with Dice Score or Jaccard Index
Source: arXiv:2010.13499 source file (2020-10-26)
Supplement: Supplementary file 5 [file l1vsl2_stderr.tex]

\begin{tabularx}{\linewidth}{llXYYYYYYY}
    \toprule
         & Loss & \multicolumn{1}{l}{\lapbox[0.5\width]{0.5em}{\emph{Data} $\rightarrow$}} & BR18 & IS17 & IS18 & MO17 & PO18 & WM17 & WM17\textsuperscript{DM} \\
    \midrule
    \parbox[t]{1mm}{\centering\multirow{2}{*}{\rotatebox[origin=c]{90}{Dice}}}
      & $L^1$   & &  0.006 &  0.034 &  0.027 &  0.003 &  0.009 & 0.019 & 0.019 \\
      & $L^2$   & &  0.006 &  0.037 &  0.027 &  0.002 &  0.011   & 0.019 & 0.020\\
    \midrule
    \parbox[t]{1mm}{\centering\multirow{2}{*}{\rotatebox[origin=c]{90}{Jacc.}}}
      & $L^1$   & &  0.008 &  0.027 &  0.023 &  0.004 &  0.009 & 0.021 & 0.021 \\
      & $L^2$   & &  0.008 &  0.029 &  0.024 &  0.004 &  0.011   & 0.021 & 0.023 \\
         
    \bottomrule
\end{tabularx}
