# Supplementary material for: Optimization for Medical Image Segmentation: Theory and Practice when evaluating with Dice Score or Jaccard Index
Source: arXiv:2010.13499 source file (2020-10-26)
Supplement: Supplementary file 6 [file multiclass_results_stderr.tex]

\begin{tabularx}{\linewidth}{llXYY|YYY}
    \toprule
    & & \multicolumn{1}{r}{\lapbox[\width]{1em}{\emph{group} $\rightarrow$}} & \multicolumn{2}{c}{CE-based} & \multicolumn{3}{c}{Metric-sensitive} \\
    \midrule
    & Type & \multicolumn{1}{r}{\lapbox[\width]{1em}{\emph{loss} $\rightarrow$}} & CE & wCE & sDice & sJaccard & Lov\'{a}sz \\
    \midrule
    \parbox[t]{7mm}{\centering\multirow{4}{*}{\rotatebox[origin=c]{90}{Dice}}} 
    & All & & 0.011 & 0.012 & 0.010 & 0.010 & 0.010 \\
    & WT  & & 0.008 & 0.009 & 0.007 & 0.007 & 0.007 \\
    & TC  & & 0.014 & 0.016 & 0.013 & 0.014 & 0.014 \\
    & ET  & & 0.020 & 0.019 & 0.017 & 0.017 & 0.018 \\
    \midrule
    \parbox[t]{7mm}{\centering\multirow{4}{*}{\rotatebox[origin=c]{90}{Jaccard}}}
    & All    & & 0.010 & 0.012 & 0.010 & 0.010 & 0.010 \\
    & WT     & & 0.010 & 0.010 & 0.009 & 0.008 & 0.008 \\
    & TC     & & 0.013 & 0.016 & 0.014 & 0.014 & 0.014 \\
    & ET     & & 0.018 & 0.018 & 0.016 & 0.016 & 0.016 \\
    \bottomrule
\end{tabularx}
