# Supplementary material for: Optimization for Medical Image Segmentation: Theory and Practice when evaluating with Dice Score or Jaccard Index
Source: arXiv:2010.13499 source file (2020-10-26)
Supplement: Supplementary file 7 [file multiclass_tversky_fmeasures.tex]

\begin{tabularx}{\linewidth}{lsXYYYYYYYYY}
    \toprule
    & Dataset & \multicolumn{1}{r}{\lapbox[\width]{1em}{\emph{$\alpha/\beta$} $\rightarrow$}} & 0.1/0.9 & 0.2/0.8 & 0.3/0.7 & 0.4/0.6 & 0.5/0.5 & 0.6/0.4 & 0.7/0.3 & 0.8/0.2 & 0.9/0.1 \\
    \midrule
    \parbox[t]{7mm}{\centering\multirow{5}{*}{\rotatebox[origin=c]{90}{BR18}}} 
    & F0.5 & & 0.739 & 0.806 & 0.841 & 0.853 & 0.878 & 0.890 & 0.896 & 0.894 & 0.879 \\
    & F1.0 & & 0.801 & 0.844 & 0.859 & 0.863 & 0.870 & 0.867 & 0.857 & 0.831 & 0.787 \\
    & F1.5 & & 0.850 & 0.874 & 0.875 & 0.873 & 0.867 & 0.855 & 0.837 & 0.798 & 0.741 \\ %old model
    & F2.0 & & 0.882 & 0.893 & 0.885 & 0.880 &  0.867 & 0.850 & 0.827 & 0.782 & 0.719 \\
    \midrule
    \parbox[t]{7mm}{\centering\multirow{5}{*}{\rotatebox[origin=c]{90}{IS17}}} 
    & F0.5 & & 0.316 & 0.318 & 0.358 & 0.372 & 0.368 & 0.367 & 0.387 & 0.382 & 0.363 \\
    & F1.0 & & 0.352 & 0.345 & 0.374 & 0.374 & 0.362 & 0.346 & 0.356 & 0.345 & 0.293 \\
    & F1.5 & & 0.398 & 0.384 & 0.402 & 0.393 & 0.378 & 0.351 & 0.360 & 0.342 & 0.274 \\ %old model
    & F2.0 & & 0.439 & 0.420 & 0.430 & 0.415 &  0.396 & 0.362 & 0.372 & 0.348 & 0.270 \\
    \midrule
    \parbox[t]{7mm}{\centering\multirow{5}{*}{\rotatebox[origin=c]{90}{IS18}}} 
    & F0.5 & & nan &          nan &          nan &          nan &  nan &          nan &          nan &          nan &          nan \\
    & F1.0 & & nan &          nan &          nan &          nan &  nan &          nan &          nan &          nan &          nan \\
    & F1.5 & & nan &          nan &          nan &          nan &  nan &          nan &          nan &          nan &          nan \\
    & F2.0 & & nan &          nan &          nan &          nan &  nan &          nan &          nan &          nan &          nan \\
    \midrule
    \parbox[t]{7mm}{\centering\multirow{5}{*}{\rotatebox[origin=c]{90}{MO17}}} 
    & F0.5 & & 0.866 & 0.900 & 0.918 & 0.930 & 0.943 & 0.948 & 0.951 & 0.954 & 0.948 \\
    & F1.0 & & 0.907 & 0.928 & 0.936 & 0.941 & 0.944 & 0.942 & 0.938 & 0.932 & 0.902 \\
    & F1.5 & & 0.936 & 0.947 & 0.949 & 0.948 & 0.945 & 0.940 & 0.930 & 0.919 & 0.876 \\ %old model
    & F2.0 & & 0.954 & 0.959 & 0.957 & 0.953 &  0.946 & 0.939 & 0.926 & 0.913 & 0.862 \\
    \midrule
    \parbox[t]{7mm}{\centering\multirow{5}{*}{\rotatebox[origin=c]{90}{PO18}}} 
    & F0.5 & & 0.610 & 0.630 & 0.639 & 0.647 & 0.664 & 0.656 & 0.663 & 0.657 & 0.651 \\
    & F1.0 & & 0.610 & 0.619 & 0.622 & 0.624 & 0.656 & 0.629 & 0.625 & 0.608 & 0.586 \\
    & F1.5 & & 0.622 & 0.623 & 0.623 & 0.620 & 0.660 & 0.623 & 0.612 & 0.589 & 0.559 \\ %old model
    & F2.0 & & 0.633 & 0.629 & 0.627 & 0.621 & 0.665 & 0.623 & 0.607 & 0.582 & 0.547 \\
    \bottomrule
\end{tabularx}
