# Supplementary material for: Optimization for Medical Image Segmentation: Theory and Practice when evaluating with Dice Score or Jaccard Index
Source: arXiv:2010.13499 source file (2020-10-26)
Supplement: Supplementary file 9 [file multiclass_tversky_stderr.tex]

% Results for new model:
\begin{tabularx}{\linewidth}{lsXYYYYYYYYY|YY}
    \toprule
    & Type & \multicolumn{1}{r}{\lapbox[\width]{1em}{\emph{$\alpha/\beta$} $\rightarrow$}} & 0.1/0.9 & 0.2/0.8 & 0.3/0.7 & 0.4/0.6 & 0.5/0.5 & 0.6/0.4 & 0.7/0.3 & 0.8/0.2 & 0.9/0.1 & 0.75/0.75 & 1.0/1.0\\
    \midrule
    \parbox[t]{7mm}{\centering\multirow{4}{*}{\rotatebox[origin=c]{90}{Dice}}} 
&All &        &        0.009 &        0.009 &        0.009 &        0.009 & 0.010 &        0.010 &        0.010 &        0.010 &        0.010 &        0.010 & 0.010 \\
&WT &        &        0.007 &        0.007 &        0.006 &        0.007 & 0.007 &        0.007 &        0.007 &        0.007 &        0.008 &        0.007 & 0.007 \\
&TC &        &        0.012 &        0.011 &        0.012 &        0.012 & 0.013 &        0.013 &        0.014 &        0.014 &        0.014 &        0.013 & 0.014 \\
&ET &        &        0.016 &        0.016 &        0.017 &        0.017 & 0.017 &        0.017 &        0.018 &        0.017 &        0.016 &        0.018 & 0.017 \\
    \midrule
    \parbox[t]{7mm}{\centering\multirow{4}{*}{\rotatebox[origin=c]{90}{Jaccard}}}
&All &        &        0.008 &        0.009 &        0.009 &        0.010 & 0.010 &        0.010 &        0.010 &        0.010 &        0.010 &        0.010 & 0.010 \\
&WT &        &        0.009 &        0.008 &        0.008 &        0.008 & 0.009 &        0.008 &        0.009 &        0.009 &        0.010 &        0.008 & 0.008 \\
&TC &        &        0.012 &        0.012 &        0.013 &        0.013 & 0.014 &        0.014 &        0.014 &        0.014 &        0.014 &        0.014 & 0.014 \\
&ET &        &        0.014 &        0.014 &        0.015 &        0.016 & 0.016 &        0.016 &        0.016 &        0.015 &        0.015 &        0.016 & 0.016 \\
    \bottomrule
\end{tabularx}
