# Supplementary material for: Optimization for Medical Image Segmentation: Theory and Practice when evaluating with Dice Score or Jaccard Index
Source: arXiv:2010.13499 source file (2020-10-26)
Supplement: Supplementary file 10 [file tversky_fmeasures.tex]

\begin{tabularx}{\linewidth}{lsXYYYYYYYYY|YY}
    \toprule
    & Measure & \multicolumn{1}{r}{\lapbox[\width]{1em}{\emph{$\alpha/\beta$} $\rightarrow$}} & 0.1/0.9 & 0.2/0.8 & 0.3/0.7 & 0.4/0.6 & 0.5/0.5 & 0.6/0.4 & 0.7/0.3 & 0.8/0.2 & 0.9/0.1 & 0.75/0.75 & 1.0/1.0 \\
    \midrule
    \parbox[t]{7mm}{\centering\multirow{5}{*}{\rotatebox[origin=c]{90}{BR18}}} 
    & F0.5 & & \textit{0.739} & 0.806 & 0.841 & 0.853 & 0.878 & 0.890 & \cellcolor{gray!50}0.896 & \cellcolor{gray!50}0.894 & 0.879 &  0.878 & 0.877 \\
    & F1.0 & & 0.801 & 0.844 & 0.859 & 0.863 & \cellcolor{gray!50}0.870 & \cellcolor{gray!50}0.867 & 0.857 & 0.831 & \textit{0.787} &  \cellcolor{gray!50}0.871 & \cellcolor{gray!50}0.868 \\
    & F1.5 & & 0.850 & \cellcolor{gray!50}0.874 & \cellcolor{gray!50}0.875 & \cellcolor{gray!50}0.873 & 0.867 & 0.855 & 0.837 & 0.798 & \textit{0.741} &  0.869 & 0.865 \\
    & F2.0 & & 0.882 & \cellcolor{gray!50}0.893 & 0.885 & 0.880 & 0.867 & 0.850 & 0.827 & 0.782 & \textit{0.719} &  0.869 & 0.865 \\
    \midrule
    \parbox[t]{7mm}{\centering\multirow{5}{*}{\rotatebox[origin=c]{90}{IS17}}} 
    & F0.5 & & 0.316 & 0.318 & \cellcolor{gray!50}0.358 & \cellcolor{gray!50}0.372 & \cellcolor{gray!50}0.368 & \cellcolor{gray!50}0.367 & \cellcolor{gray!50}0.387 & \cellcolor{gray!50}0.382 & \cellcolor{gray!50}0.363 &  0.367 & 0.362 \\
    & F1.0 & & \cellcolor{gray!50}0.352 & 0.345 & \cellcolor{gray!50}0.374 & \cellcolor{gray!50}0.374 & \cellcolor{gray!50}0.362 & 0.346 & \cellcolor{gray!50}0.356 & \cellcolor{gray!50}0.345 & 0.293 &  \cellcolor{gray!50}0.371 & \cellcolor{gray!50}0.363 \\
    & F1.5 & & \cellcolor{gray!50}0.398 & \cellcolor{gray!50}0.384 & \cellcolor{gray!50}0.402 & \cellcolor{gray!50}0.393 & \cellcolor{gray!50}0.378 & 0.351 & 0.360 & 0.342 & \textit{0.274} &  \cellcolor{gray!50}0.394 & \cellcolor{gray!50}0.384 \\
    & F2.0 & & \cellcolor{gray!50}0.439 & \cellcolor{gray!50}0.420 & \cellcolor{gray!50}0.430 & \cellcolor{gray!50}0.415 & \cellcolor{gray!50}0.396 & 0.362 & 0.372 & 0.348 & \textit{0.270} &  \cellcolor{gray!50}0.419 & \cellcolor{gray!50}0.408 \\
    \midrule
    \parbox[t]{7mm}{\centering\multirow{5}{*}{\rotatebox[origin=c]{90}{IS18}}} 
    & F0.5 & & \textit{0.411} & 0.468 & 0.495 & 0.516 & \cellcolor{gray!50}0.528 & 0.528 & \cellcolor{gray!50}0.539 & \cellcolor{gray!50}0.543 & \cellcolor{gray!50}0.530 &  0.521 & 0.520 \\
    & F1.0 & & 0.481 & 0.522 & 0.533 & \cellcolor{gray!50}0.540 & \cellcolor{gray!50}0.538 & \cellcolor{gray!50}0.527 & 0.519 & 0.490 & \textit{0.445} &  0.528 & 0.528 \\
    & F1.5 & & 0.551 & \cellcolor{gray!50}0.573 & \cellcolor{gray!50}0.571 & \cellcolor{gray!50}0.568 & 0.555 & 0.537 & 0.517 & 0.470 & \textit{0.413} &  0.544 & 0.544 \\
    & F2.0 & & \cellcolor{gray!50}0.607 & \cellcolor{gray!50}0.612 & 0.600 & 0.590 & 0.569 & 0.547 & 0.520 & 0.464 & \textit{0.399} &  0.558 & 0.558 \\
    \midrule
    \parbox[t]{7mm}{\centering\multirow{5}{*}{\rotatebox[origin=c]{90}{MO17}}} 
    & F0.5 & & \textit{0.866} & 0.900 & 0.918 & 0.930 & 0.943 & 0.948 & 0.951 & \cellcolor{gray!50}0.954 & 0.948 &  0.943 & 0.942 \\
    & F1.0 & & 0.907 & 0.928 & 0.936 & 0.941 & \cellcolor{gray!50}0.944 & \cellcolor{gray!50}0.942 & 0.938 & 0.932 & 0.902 &  \cellcolor{gray!50}0.944 & \cellcolor{gray!50}0.942 \\
    & F1.5 & & 0.936 & 0.947 & \cellcolor{gray!50}0.949 & \cellcolor{gray!50}0.948 & 0.945 & 0.940 & 0.930 & 0.919 & \textit{0.876} &  0.945 & 0.944 \\
    & F2.0 & & 0.954 & \cellcolor{gray!50}0.959 & 0.957 & 0.953 & 0.946 & 0.939 & 0.926 & 0.913 & \textit{0.862} &  0.946 & 0.945 \\
    \midrule
    \parbox[t]{7mm}{\centering\multirow{5}{*}{\rotatebox[origin=c]{90}{PO18}}} 
    & F0.5 & & \textit{0.588} & 0.609 & 0.625 & 0.644 & \cellcolor{gray!50}0.664 & \cellcolor{gray!50}0.664 & \cellcolor{gray!50}0.671 & \cellcolor{gray!50}0.669 & \cellcolor{gray!50}0.664 & 0.656 & 0.657 \\
    & F1.0 & & 0.614 & 0.628 & 0.637 & 0.647 & \cellcolor{gray!50}0.656 & \cellcolor{gray!50}0.650 & 0.647 & 0.633 & 0.611 & 0.646 & \cellcolor{gray!50}0.651 \\
    & F1.5 & & 0.643 & 0.651 & \cellcolor{gray!50}0.654 & \cellcolor{gray!50}0.658 & \cellcolor{gray!50}0.660 & 0.651 & 0.641 & 0.620 & \textit{0.591} & 0.650 & \cellcolor{gray!50}0.656 \\
    & F2.0 & & \cellcolor{gray!50}0.665 & \cellcolor{gray!50}0.669 & \cellcolor{gray!50}0.668 & \cellcolor{gray!50}0.668 & \cellcolor{gray!50}0.665 & 0.655 & 0.640 & 0.616 & \textit{0.582} & 0.655 & \cellcolor{gray!50}0.662 \\
    \midrule
    \parbox[t]{7mm}{\centering\multirow{5}{*}{\rotatebox[origin=c]{90}{WM17}}} 
    & F0.5 & & \textit{0.498} & 0.592 & 0.659 & 0.690 & 0.724 & 0.742 & \cellcolor{gray!50}0.761 & \cellcolor{gray!50}0.759 & 0.720 &  0.723 & 0.730 \\
    & F1.0 & & 0.581 & 0.649 & 0.689 & 0.700 & \cellcolor{gray!50}0.712 & 0.706 & 0.693 & 0.660 & 0.565 &  \cellcolor{gray!50}0.712 & \cellcolor{gray!50}0.712 \\
    & F1.5 & & 0.657 & 0.700 & \cellcolor{gray!50}0.718 & 0.713 & \cellcolor{gray!50}0.711 & 0.692 & 0.660 & 0.615 & \textit{0.501} &  0.712 & 0.708 \\
    & F2.0 & & 0.714 & \cellcolor{gray!50}0.736 & \cellcolor{gray!50}0.739 & 0.724 & 0.713 & 0.686 & 0.645 & 0.593 & \textit{0.472} &  0.714 & 0.708 \\
    \midrule
    \parbox[t]{7mm}{\centering\multirow{5}{*}{\rotatebox[origin=c]{90}{WM17\textsuperscript{DM}}}} 
    & F0.5 & & \textit{0.521} & 0.617 & 0.671 & 0.709 & 0.736 & \cellcolor{gray!50}0.758 & \cellcolor{gray!50}0.759 & \cellcolor{gray!50}0.752 & 0.647 &  0.731 & 0.736 \\
    & F1.0 & & 0.599 & 0.668 & 0.696 & 0.709 & \cellcolor{gray!50}0.717 & 0.706 & 0.675 & 0.628 & \textit{0.496} &  0.706 & \cellcolor{gray!50}0.714 \\
    & F1.5 & & 0.670 & \cellcolor{gray!50}0.713 & \cellcolor{gray!50}0.722 & \cellcolor{gray!50}0.717 & 0.712 & 0.682 & 0.636 & 0.574 & \textit{0.436} &  0.697 & 0.707 \\
    & F2.0 & & 0.721 & \cellcolor{gray!50}0.744 & \cellcolor{gray!50}0.739 & 0.723 & 0.712 & 0.672 & 0.618 & 0.548 & \textit{0.409} &  0.695 & 0.706 \\
    \bottomrule
\end{tabularx}
