# Supplementary material for: Optimization for Medical Image Segmentation: Theory and Practice when evaluating with Dice Score or Jaccard Index
Source: arXiv:2010.13499 source file (2020-10-26)
Supplement: Supplementary file 11 [file tversky_fmeasures_stderr.tex]

\begin{tabularx}{\linewidth}{lsXYYYYYYYYY|YY}
    \toprule
    & Measure & \multicolumn{1}{r}{\lapbox[\width]{1em}{\emph{$\alpha/\beta$} $\rightarrow$}} & 0.1/0.9 & 0.2/0.8 & 0.3/0.7 & 0.4/0.6 & 0.5/0.5 & 0.6/0.4 & 0.7/0.3 & 0.8/0.2 & 0.9/0.1 & 0.75/0.75 & 1.0/1.0 \\
    \midrule
    \parbox[t]{7mm}{\centering\multirow{5}{*}{\rotatebox[origin=c]{90}{BR18}}} 
    & F0.5 & & 0.008 & 0.007 & 0.007 & 0.007 & 0.006 & 0.005 & 0.006 & 0.006 & 0.006 &  0.006 & 0.007 \\
    & F1.0 & & 0.007 & 0.006 & 0.006 & 0.006 & 0.006 & 0.006 & 0.007 & 0.007 & 0.008 &  0.006 & 0.007 \\
    & F1.5 & & 0.006 & 0.005 & 0.006 & 0.006 & 0.006 & 0.006 & 0.007 & 0.008 & 0.009 &  0.007 & 0.007 \\
    & F2.0 & & 0.005 & 0.005 & 0.006 & 0.007 & 0.007 & 0.007 & 0.008 & 0.009 & 0.009 &  0.007 & 0.007 \\
    \midrule
    \parbox[t]{7mm}{\centering\multirow{5}{*}{\rotatebox[origin=c]{90}{IS17}}} 
    & F0.5 & & 0.034 & 0.035 & 0.039 & 0.040 & 0.037 & 0.038 & 0.038 & 0.037 & 0.036 &  0.036 & 0.037 \\
    & F1.0 & & 0.036 & 0.035 & 0.037 & 0.037 & 0.034 & 0.034 & 0.033 & 0.034 & 0.031 &  0.033 & 0.035 \\
    & F1.5 & & 0.037 & 0.036 & 0.036 & 0.036 & 0.034 & 0.033 & 0.032 & 0.034 & 0.030 &  0.033 & 0.035 \\
    & F2.0 & & 0.039 & 0.037 & 0.036 & 0.037 & 0.034 & 0.034 & 0.032 & 0.035 & 0.030 &  0.034 & 0.036 \\
    \midrule
    \parbox[t]{7mm}{\centering\multirow{5}{*}{\rotatebox[origin=c]{90}{IS18}}} 
    & F0.5 & & 0.024 & 0.026 & 0.026 & 0.027 & 0.028 & 0.028 & 0.029 & 0.029 & 0.030 &  0.028 & 0.028 \\
    & F1.0 & & 0.025 & 0.026 & 0.026 & 0.026 & 0.027 & 0.027 & 0.027 & 0.027 & 0.027 &  0.027 & 0.027 \\
    & F1.5 & & 0.025 & 0.026 & 0.026 & 0.026 & 0.027 & 0.027 & 0.027 & 0.026 & 0.026 &  0.027 & 0.027 \\
    & F2.0 & & 0.026 & 0.026 & 0.027 & 0.026 & 0.027 & 0.027 & 0.027 & 0.026 & 0.025 &  0.027 & 0.027 \\
    \midrule
    \parbox[t]{7mm}{\centering\multirow{5}{*}{\rotatebox[origin=c]{90}{MO17}}} 
    & F0.5 & & 0.004 & 0.004 & 0.004 & 0.003 & 0.003 & 0.003 & 0.002 & 0.003 & 0.002 &  0.003 & 0.003 \\
    & F1.0 & & 0.003 & 0.003 & 0.003 & 0.003 & 0.003 & 0.003 & 0.002 & 0.003 & 0.003 &  0.002 & 0.003 \\
    & F1.5 & & 0.002 & 0.002 & 0.002 & 0.002 & 0.002 & 0.003 & 0.002 & 0.003 & 0.003 &  0.002 & 0.003 \\
    & F2.0 & & 0.002 & 0.002 & 0.002 & 0.002 & 0.002 & 0.003 & 0.002 & 0.003 & 0.004 &  0.002 & 0.003 \\
    \midrule
    \parbox[t]{7mm}{\centering\multirow{5}{*}{\rotatebox[origin=c]{90}{PO18}}} 
    & F0.5 & & 0.009 & 0.009 & 0.009 & 0.009 & 0.009 & 0.010 & 0.010 & 0.010 & 0.010 & 0.010 & 0.009 \\
    & F1.0 & & 0.009 & 0.009 & 0.009 & 0.009 & 0.009 & 0.010 & 0.010 & 0.010 & 0.010 & 0.010 & 0.010 \\
    & F1.5 & & 0.009 & 0.010 & 0.010 & 0.010 & 0.010 & 0.010 & 0.010 & 0.010 & 0.010 & 0.010 & 0.010 \\
    & F2.0 & & 0.010 & 0.010 & 0.010 & 0.010 & 0.010 & 0.010 & 0.010 & 0.010 & 0.010 & 0.010 & 0.010 \\
    \midrule
    \parbox[t]{7mm}{\centering\multirow{5}{*}{\rotatebox[origin=c]{90}{WM17}}} 
    & F0.5 & & 0.019 & 0.019 & 0.018 & 0.020 & 0.018 & 0.019 & 0.017 & 0.018 & 0.020 &  0.020 & 0.019 \\
    & F1.0 & & 0.018 & 0.018 & 0.018 & 0.018 & 0.019 & 0.020 & 0.019 & 0.020 & 0.021 &  0.019 & 0.020 \\
    & F1.5 & & 0.018 & 0.019 & 0.018 & 0.019 & 0.020 & 0.021 & 0.020 & 0.021 & 0.021 &  0.019 & 0.021 \\
    & F2.0 & & 0.017 & 0.019 & 0.019 & 0.019 & 0.021 & 0.021 & 0.021 & 0.021 & 0.020 &  0.020 & 0.021 \\ 
    \midrule
    \parbox[t]{7mm}{\centering\multirow{5}{*}{\rotatebox[origin=c]{90}{WM17\textsuperscript{DM}}}} 
    & F0.5 & & 0.018 & 0.017 & 0.018 & 0.017 & 0.017 & 0.018 & 0.019 & 0.020 & 0.032 &  0.018 & 0.018 \\
    & F1.0 & & 0.018 & 0.018 & 0.018 & 0.018 & 0.019 & 0.020 & 0.022 & 0.023 & 0.030 &  0.020 & 0.020 \\
    & F1.5 & & 0.018 & 0.018 & 0.020 & 0.020 & 0.020 & 0.022 & 0.023 & 0.024 & 0.029 &  0.021 & 0.022 \\
    & F2.0 & & 0.018 & 0.019 & 0.021 & 0.021 & 0.021 & 0.022 & 0.024 & 0.024 & 0.028 &  0.022 & 0.023 \\
    \bottomrule
\end{tabularx}
