# Supplementary material for: Optimization for Medical Image Segmentation: Theory and Practice when evaluating with Dice Score or Jaccard Index
Source: arXiv:2010.13499 source file (2020-10-26)
Supplement: Supplementary file 12 [file tversky_stderr.tex]

\begin{tabularx}{\linewidth}{lsXYYYYYYYYY|YY}
    \toprule
    & Dataset & \multicolumn{1}{r}{\lapbox[\width]{1em}{\emph{$\alpha/\beta$} $\rightarrow$}} & 0.1/0.9 & 0.2/0.8 & 0.3/0.7 & 0.4/0.6 & 0.5/0.5 & 0.6/0.4 & 0.7/0.3 & 0.8/0.2 & 0.9/0.1 & 0.75/0.75 & 1.0/1.0 \\
    \midrule
    \parbox[t]{7mm}{\centering\multirow{5}{*}{\rotatebox[origin=c]{90}{Dice}}} 
    &BR18 &        &        0.007 &        0.006 &        0.006 &        0.006 & 0.006 &        0.006 &        0.007 &        0.007 &        0.008 &        0.006 & 0.007 \\
    &IS17 &        &        0.036 &        0.035 &        0.037 &        0.037 & 0.034 &        0.034 &        0.033 &        0.034 &        0.031 &        0.033 & 0.035 \\
    &IS18 &        &        0.025 &        0.026 &        0.026 &        0.026 & 0.027 &        0.027 &        0.027 &        0.027 &        0.027 &        0.027 & 0.027 \\
    &MO18 &        &        0.003 &        0.003 &        0.003 &        0.003 & 0.003 &        0.003 &        0.002 &        0.003 &        0.003 &        0.002 & 0.003 \\
    &PO18 &        &        0.009 &        0.009 &        0.009 &        0.009 & 0.009 &        0.010 &        0.010 &        0.010 &        0.010 &          0.010 & 0.010 \\
    &WM17 &        &        0.018 &        0.018 &        0.018 &        0.018 & 0.019 &        0.020 &        0.019 &        0.020 &        0.021 &        0.019 & 0.020 \\
    &WM17\textsuperscript{DM} &        &        0.018 &        0.018 &        0.018 &        0.018 & 0.019 &        0.020 &        0.022 &        0.023 &        0.030 &        0.020 & 0.020 \\
    \midrule
    \parbox[t]{7mm}{\centering\multirow{5}{*}{\rotatebox[origin=c]{90}{Jaccard}}}
    &BR18 &        &        0.008 &        0.007 &        0.008 &        0.008 & 0.008 &        0.007 &        0.008 &        0.009 &        0.010 &        0.008 & 0.008 \\
    &IS17 &        &        0.028 &        0.027 &        0.028 &        0.029 & 0.027 &        0.026 &        0.025 &        0.025 &        0.022 &        0.026 & 0.028 \\
    &IS18 &        &        0.022 &        0.023 &        0.023 &        0.023 & 0.023 &        0.023 &        0.023 &        0.023 &        0.022 &        0.024 & 0.024 \\
    &MO18 &        &        0.004 &        0.004 &        0.004 &        0.004 & 0.004 &        0.004 &        0.003 &        0.004 &        0.004 &        0.003 & 0.004 \\
    &PO18 &        &        0.008 &        0.009 &        0.009 &        0.009 & 0.009 &        0.009 &        0.009 &        0.009 &        0.009 &          0.009 & 0.009 \\
    &WM17 &        &        0.017 &        0.019 &        0.019 &        0.021 & 0.021 &        0.021 &        0.021 &        0.021 &        0.019 &        0.021 & 0.022 \\
    &WM17\textsuperscript{DM} &        &        0.017 &        0.018 &        0.020 &        0.021 & 0.021 &        0.022 &        0.023 &        0.023 &        0.026 &        0.022 & 0.022 \\
    \bottomrule
\end{tabularx}
